# Supplementary material for: What and When to Look?: Temporal Span Proposal Network for Video Relation Detection
Source: arXiv:2107.07154 source file (2022-10-05)
Supplement: Supplementary file 1 [file 06appendix.tex]

% if have a single appendix:
%\appendix[Proof of the Zonklar Equations]
% or
%\appendix  % for no appendix heading
% do not use \section anymore after \appendix, only \section*
% is possibly needed

% use appendices with more than one appendix
% then use \section to start each appendix
% you must declare a \section before using any
% \subsection or using \label (\appendices by itself
% starts a section numbered zero.)
%
\appendices
